# Supplementary material for: Empowering high-dimensional quantum computing by traversing the dual bosonic ladder
Source: arXiv:2312.17741 source file (2023-12-29)
Supplement: Supplementary file 1 [file S12.tex]

\subsection{Supplementary Note 9 --
Fabrication}

The comprehensive fabrication process and calibration procedures have been extensively documented in \cite{kreikebaum2020superconducting}, and a concise overview will be provided herein.

The device was fabricated on a high-resistivity silicon wafer ($\rho > 10 \text{k}\Omega\text{-cm}$) with Niobium (Nb) and Aluminum (Al). After cleaning the wafer with piranha (mixture of sulfuric acid and hydrogen peroxide heated to $120^\circ \text{C}$) and hydrofluoric acid (HF) to remove the organics and silicon oxide, a 200-nm layer of Nb was deposited through sputtering. Subsequently, the superconducting circuit components, excluding the junctions, were defined by the photo-lithography technique and reactive-ion etching. It is noteworthy that deliberate over-etching of the silicon substrate was implemented to prevent short circuits and minimize dielectric loss.

Subsequent to this, the wafer underwent cleaning with buffered oxide etch (BOE) solvent in preparation for the fabrication of Josephson junctions. The Josephson junctions were precisely defined through e-beam lithography and deposited via a 3-angle e-beam evaporation of Aluminum (Al) films, employing the Manhattan-style technique. To optimize the adhesion between the substrate and the Al films, a mild plasma cleaning process was applied prior to the deposition of the Al film. This procedure served to eliminate e-beam resist residues and enhance the adhesion. The galvanic connection between the Josephson junctions and their respective capacitor pads was established using an Argon ion-milling band-aid process.

Finally, the fabricated wafer was coated with methyl methacrylate (MMA) resist to protect it before dicing. Following dicing, the chips were cleaned with N-methylpyrrolidone (NMP) at $80^\circ \text{C}$ and packaged in a copper box for testing in the dilute refrigerators.

\textbf{\textcolor{blue}{Long}}
