# Supplementary material for: Empowering high-dimensional quantum computing by traversing the dual bosonic ladder
Source: arXiv:2312.17741 source file (2023-12-29)
Supplement: Supplementary file 2 [file S4.tex]

\subsection{Supplementary Note 4 --
Quantum process tomography of two-photon interactions}

\textbf{\textcolor{blue}{Noah}}
