# Supplementary material for: Empowering high-dimensional quantum computing by traversing the dual bosonic ladder
Source: arXiv:2312.17741 source file (2023-12-29)
Supplement: Supplementary file 3 [file S5.tex]

\subsection{Supplementary Note 5 --
CnZ gate: Calibration}

\textbf{\textcolor{blue}{Long}}
