# Supplementary material for: Empowering high-dimensional quantum computing by traversing the dual bosonic ladder
Source: arXiv:2312.17741 source file (2023-12-29)
Supplement: Supplementary file 4 [file S8.tex]

\subsection{Supplementary Note 8 --
Density Matrix Purification}

\textbf{\textcolor{blue}{Long}}
